# Supplementary material for: L-DAWA: Layer-wise Divergence Aware Weight Aggregation in Federated Self-Supervised Visual Representation Learning
Source: arXiv:2307.07393 source file (2023-07-14)
Supplement: Supplementary file 1 [file 6_Appendix.tex]

% \documentclass[10pt,twocolumn,letterpaper]{article}
% \usepackage{iccv}
% \usepackage{times}
% \usepackage{epsfig}
% \usepackage{graphicx}
% \usepackage{amsmath}
% \usepackage{amssymb}

% \usepackage{booktabs}
% \usepackage{url}
% \usepackage{multirow}
% \usepackage{caption}
% \usepackage{subcaption}
% \usepackage{pifont}
% \usepackage{algorithm}
% \usepackage{array}
% \usepackage[noend]{algpseudocode}
% % \usepackage{pifont}
% % \usepackage{blindtext}

% % \usepackage{subfiles} % Best loaded last in the preamble
% % \usepackage{hyperref}
% % \usepackage[capitalize]{cleveref}
% % \crefname{section}{Sec.}{Secs.}
% % \Crefname{section}{Section}{Sections}
% % \Crefname{table}{Table}{Tables}
% % \crefname{table}{Tab.}{Tabs.}
% % Include other packages here, before hyperref.

% % If you comment hyperref and then uncomment it, you should delete
% % egpaper.aux before re-running latex.  (Or just hit 'q' on the first latex
% % run, let it finish, and you should be clear).
% \usepackage[pagebackref=true,breaklinks=true,letterpaper=true,colorlinks,bookmarks=false]{hyperref}

% % \iccvfinalcopy % *** Uncomment this line for the final submission

% \def\iccvPaperID{9974} % *** Enter the ICCV Paper ID here
% \def\httilde{\mbox{\tt\raisebox{-.5ex}{\symbol{126}}}}

% % Pages are numbered in submission mode, and unnumbered in camera-ready
% \ificcvfinal\pagestyle{empty}\fi

% \begin{document}

\section{Appendix}
\label{sec:appendix}

\subsection{SimCLR vs Barlow Twins Loss Function}
\begin{equation}
   L_{SimCLR} = u^{T}v^{+}/\tau - log\sum_{v \in \{v^{+},v^{-}\}} exp(u^{T}v/\tau)  
\end{equation}
The above equation represents the NT-Xent (Normalized Temperature-scaled Cross Entropy) loss function as proposed in \cite{chen2020simple}. The input $u^{T}$, $v^{+}$, and $v^{-}$ are $l_{2}$ normalized. $\tau$ is a temperature coefficient.
\begin{equation}
 L_{Barlow Twins} = \sum_{i}(1-C_{ii})^{2} + \lambda \sum_{i}\sum_{j\neq i}C_{ij}^{2}
\end{equation}
In the above equation, $C$ represents the cross-correlation matrix computed on the output features of the two identical networks along the batch dimension, as illustrated in \cite{zbontar2021barlow}. $C_{ii}$ represents the diagonal elements of the cross-correlation matrix while $C_{ij}$ represents the off-diagonal elements of the cross-correlation matrix. $\lambda$ is a positive hyperparameter that controls the trade-off between the first term (invariance) and the second term (redundancy reduction).
\subsection{Effectiveness of $\delta$ in L-DAWA}
We find that the \textit{angular measure of divergence} (i.e., $\delta$) between the local clients model and the global model plays an important role in determining the trajectory  of the final global model. In Table \ref{tab:ablation_ldawa}, we show that without $\delta$, L-DAWA results in sub-optimal performance. The results in Table \ref{tab:ablation_ldawa} imply that for prolonged training in FL, both FedAvg and L-DAWA(without $\delta$) will result in sub-optimal performance. We also find that without $\delta$, L-DAWA reduces to FairAvg \cite{michieli2021all}, (i.e., $w^{r+1}_{g} = \frac{1}{K}\sum^{K}_{k=1}w^{r}_{k}$). However, one can see in Table \ref{tab:ablation_ldawa} that even treating all the clients with the same weighting (i.e., $\frac{1}{K}$), the results are sub-optimal. 
\begin{table}[ht]
    \centering
   
    % \resizebox{\columnwidth}{!}{
    \begin{tabular}{l|ccc}
    \hline
         Method &  E1 & E5 & E10\\
         \toprule
         FedAvg &  50.92 & 65.05 & 71.07  \\
         L-DAWA w/o $\delta$  & 50.33 & 64.09 & 70.31 \\
         L-DAWA w/  $\delta$  & \textbf{60.29} &\textbf{ 70.65} & \textbf{75.60}\\
       
         \bottomrule
         
    \end{tabular}
    % }
     \caption{Ablation study: Each method is pre-trained with SimCLR  on the Non-iid version of CIFAR-10 under the \textit{cross-silo (K=10)} settings for $R=200$ rounds.}
    \label{tab:ablation_ldawa}
    \end{table}

\subsection{Properties of L-DAWA}
% \subsection{Properties of M-DAWA and L-DAWA}
We find that L-DAWA intrinsically provides significant performance improvement in \textit{cross-silo} settings. Such performance improvement signifies the importance of introducing divergence control during weight aggregation. One can see from Table \ref{tab:sota_full_comparison}, that L-DAWA  provides a lightweight aggregation method that is unbiased and independent of the metadata. L-DAWA provides layer-wise divergence control at the server, unlike FedU which provides partial divergence control for only the predictor network on the client side. One can further note from Table \ref{tab:sota_full_comparison} that FedAvg, Loss, and FedU equally treat all the layers of the client's model by multiplying it with a constant coefficient. In contrast, L-DAWA treats each layer of the client's model by the measure of divergence that varies from layer to layer.

The current state-of-the-art aggregation methods (FedAvg, Loss, and FedU) can be improved by introducing a measure of the model quality based on \textit{angular measure of divergence} as shown in Table \ref{tab:sota_full_comparison}. We note that individual bias toward sample size as in FedAvg and FedU, Local Loss in Loss aggregation strategies is effectively mitigated by introducing \textit{angular measure of divergence} in these methods resulting in an improved and fair performance for both contrastive (SimCLR) and non-contrastive (Barlow Twins) SSL approaches.  

\begin{table*}[h]
    \centering
    
    \resizebox{2\columnwidth}{!}{
    \begin{tabular}{lcccccc|cc|cccc|cc}
    \toprule
         Method & Metadata & Type & Bias & Model Quality & Div.Control & Agg.Rule & \multicolumn{2}{c}{W.Coefficient} &\multicolumn{6}{|c}{\%Acc. Cross-Silo} \\
         \cline{8-15}
         & & & & & &  & \multirow{2}{*}{Type} & \multirow{2}{*}{Nature} &\multicolumn{2}{|c|}{CIFAR-10} & \multicolumn{2}{|c}{CIFAR-100} & \multicolumn{2}{c}{Tiny ImageNet}  \\
         \cline{10-15}
         & & & &  &  &  &  & & SimCLR & Barlow Twins & SimCLR & Barlow Twins & SimCLR & Barlow Twins \\
         \hline
         FedAvg & \cmark & Sample Size & \cmark& \xmark & None & W.Avg & Sample Prob. & Const. & 71.07  & 65.02 & 43.85 & 35.70 & 32.92 & 15.40\\
         Loss & \cmark & Local Loss &\cmark & \xmark & None & W.Avg & Local Loss & Const. & 71.34  & 57.12 & 44.69  &34.76 & 33.37 & 12.24 \\
         FedU & \cmark & Sample Size & \cmark & Partial & Partial &  W.Avg & Sample Prob. & Const.  &  70.36 &64.55 & 44.31 & 35.25 & 32.63 & 15.16\\
         
        %  L-DAWA & \xmark & None & \xmark &\cmark & Layer-wise & Seq.W.Avg & Layer-Wise Div. & Var. & \underline{75.25} & \textbf{69.41}  & \underline{49.25} & \underline{41.35} \\
        \hline
         L-DAWA & \xmark & None & \xmark &\cmark & Layer-wise & W.Avg & Layer-Wise Div. & Var. & 75.60 &  69.31& 49.88 & 41.85 & 37.22 & 21.47 \\
         L-DAWA$_{FedAvg}$ & \cmark & Sample Size & \cmark & \cmark & Layer-wise & W.Avg & Layer-Wise Div.+ Sample Prob. & Var. & 75.72 & \textbf{69.92} & 49.99 & 41.49 & 36.97 & 21.58 \\
         L-DAWA$_{Loss}$ & \cmark & Local Loss & \cmark & \cmark & Layer-wise & W.Avg & Layer-Wise Div.+ Local Loss & Var. & \textbf{76.55} & 69.46 & 50.29 & \textbf{41.89} & & 11.90 \\
         L-DAWA$_{FedU}$ & \cmark & Sample Size & \cmark & \cmark & Layer-wise & W.Avg & Layer-Wise Div.+ Sample Size & Var. & 76.23 & 69.50 & \textbf{50.59} & 41.72 & 37.12 &21.80 \\
         
         \hline
    \end{tabular}
    }
    \caption{Comparison of state-of-the-art aggregation methods. "Agg.", "Div.", "W.Avg", "Seq.", "W.Scalar", "Prob.", "Const.", "Var." stands for Aggregation, Divergence, Weighted Average, Sequential, Weighting Scalar, Probability, Constant, and Variable, respectively.} 
    \label{tab:sota_full_comparison}
\end{table*}

\subsection{Loss landscape of L-DAWA}
We further explore the effects of L-DAWA on the model's global loss landscape and the global optimization trajectories under the \textit{cross-silo} settings with SimCLR. For this purpose, we explore the loss landscape and optimization trajectories of Loss, FedU, L-DAWA$_{FedAvg}$, L-DAWA$_{Loss}$, and L-DAWA$_{FedU}$. Interestingly, we find that the loss landscape of Loss and FedU (Figure \ref{fig:Optimization-supp} (a-b)) is more chaotic and the global optimization trajectory fell into a narrow local minimum leading to sub-optimal performance. Interestingly, when L-DAWA is introduced into these aggregation methods, the global optimization trajectory ends up in a much wider basin of attraction in the loss landscape resulting in improved performance (Figure \ref{fig:Optimization-supp}(c-d)).

\begin{figure*}
\centering
\begin{subfigure}{0.2\linewidth}
    \centering
    \includegraphics[scale=0.35]{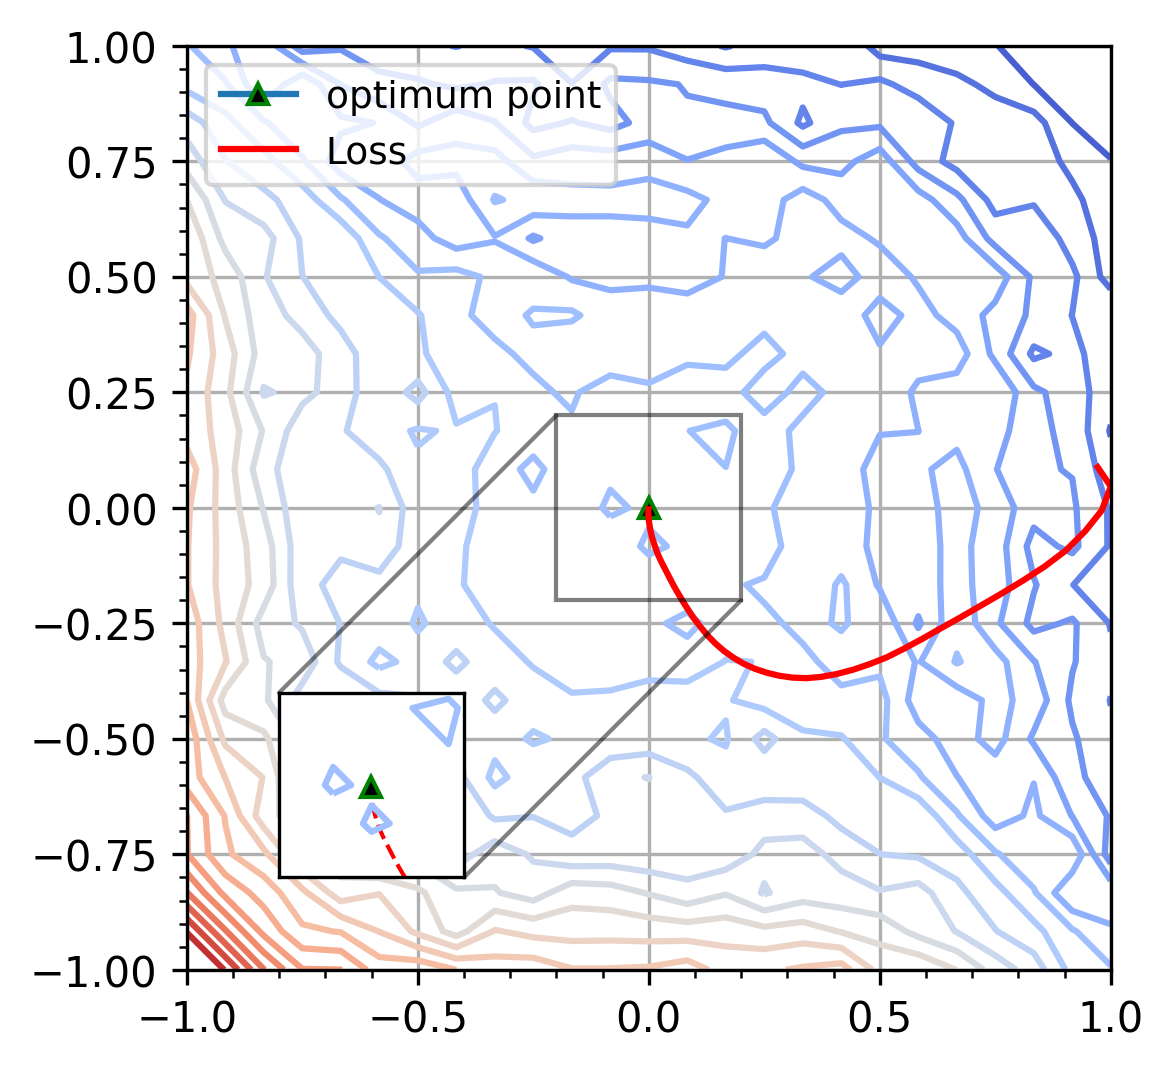}
    \caption{Loss}
\end{subfigure}%
\begin{subfigure}{0.2\linewidth}
    \centering
    \includegraphics[scale=0.35]{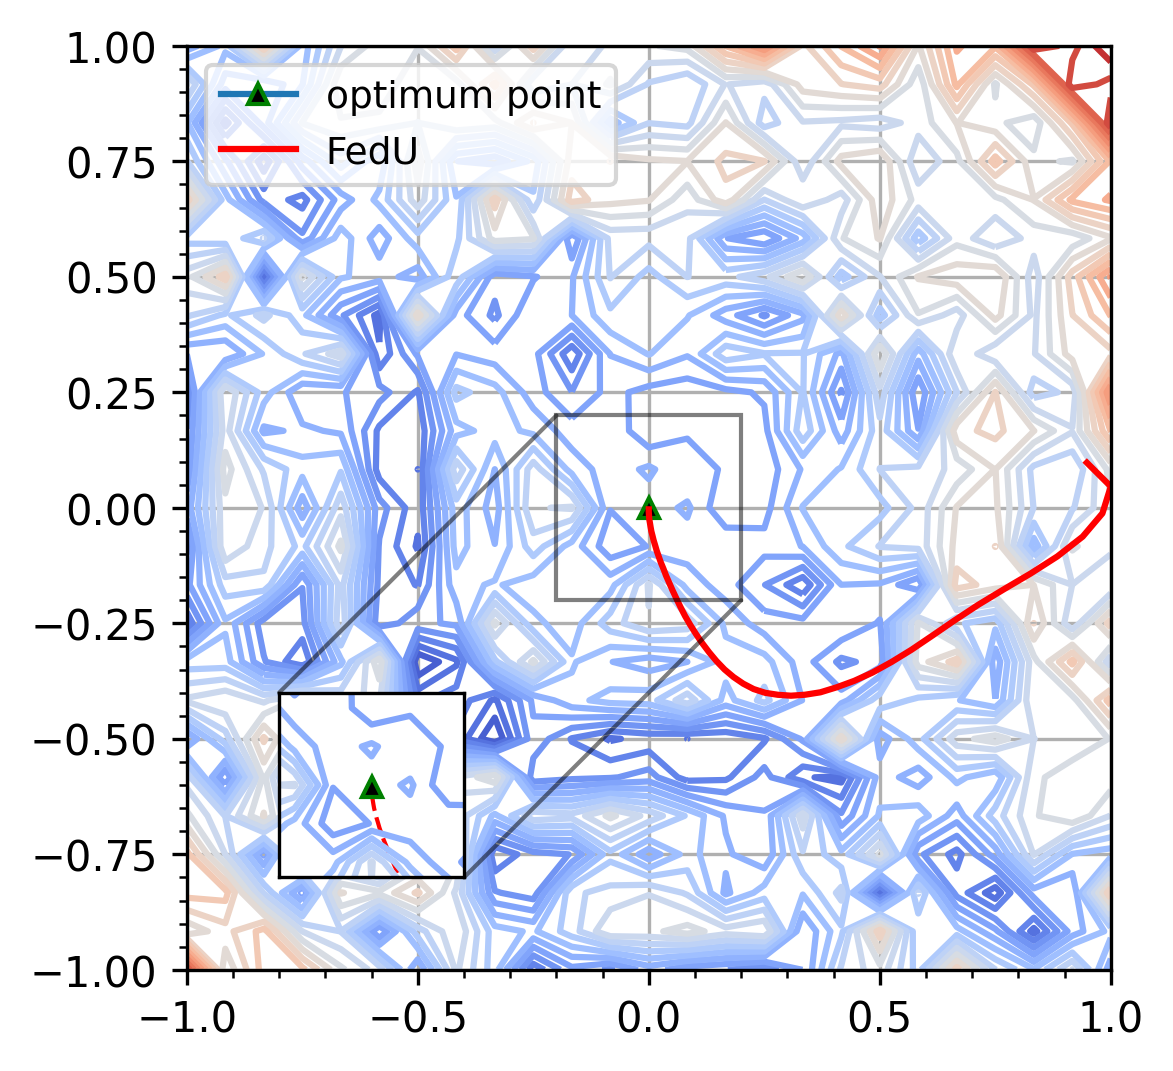}
    \caption{FedU}
\end{subfigure}%
\begin{subfigure}{0.2\linewidth}
        \centering
    \includegraphics[scale=0.35]{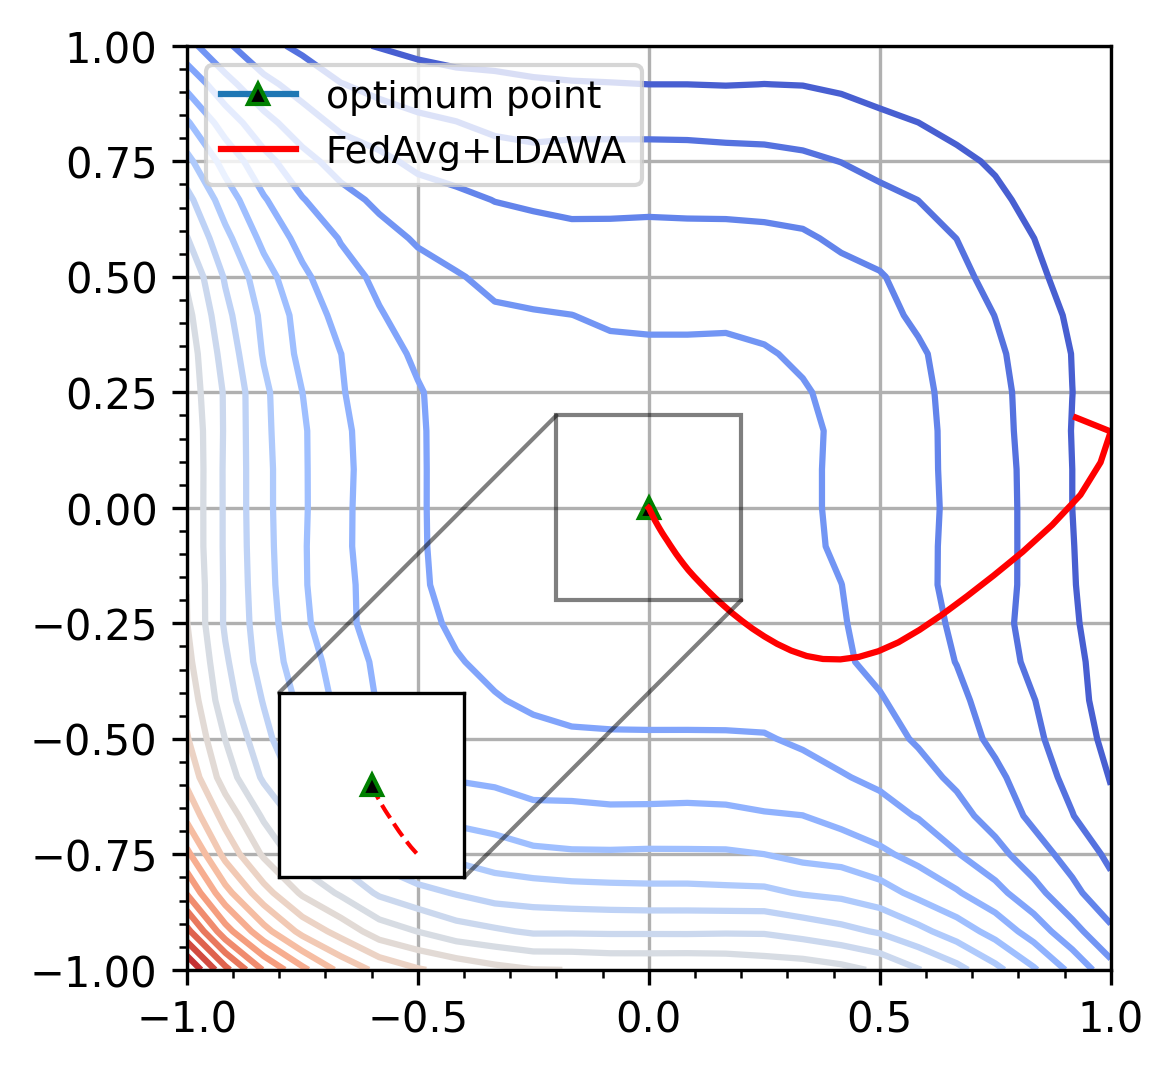}
    \caption{FedAvg+L-DAWA}
\end{subfigure}%
\begin{subfigure}{0.2\linewidth}
        \centering
    \includegraphics[scale=0.35]{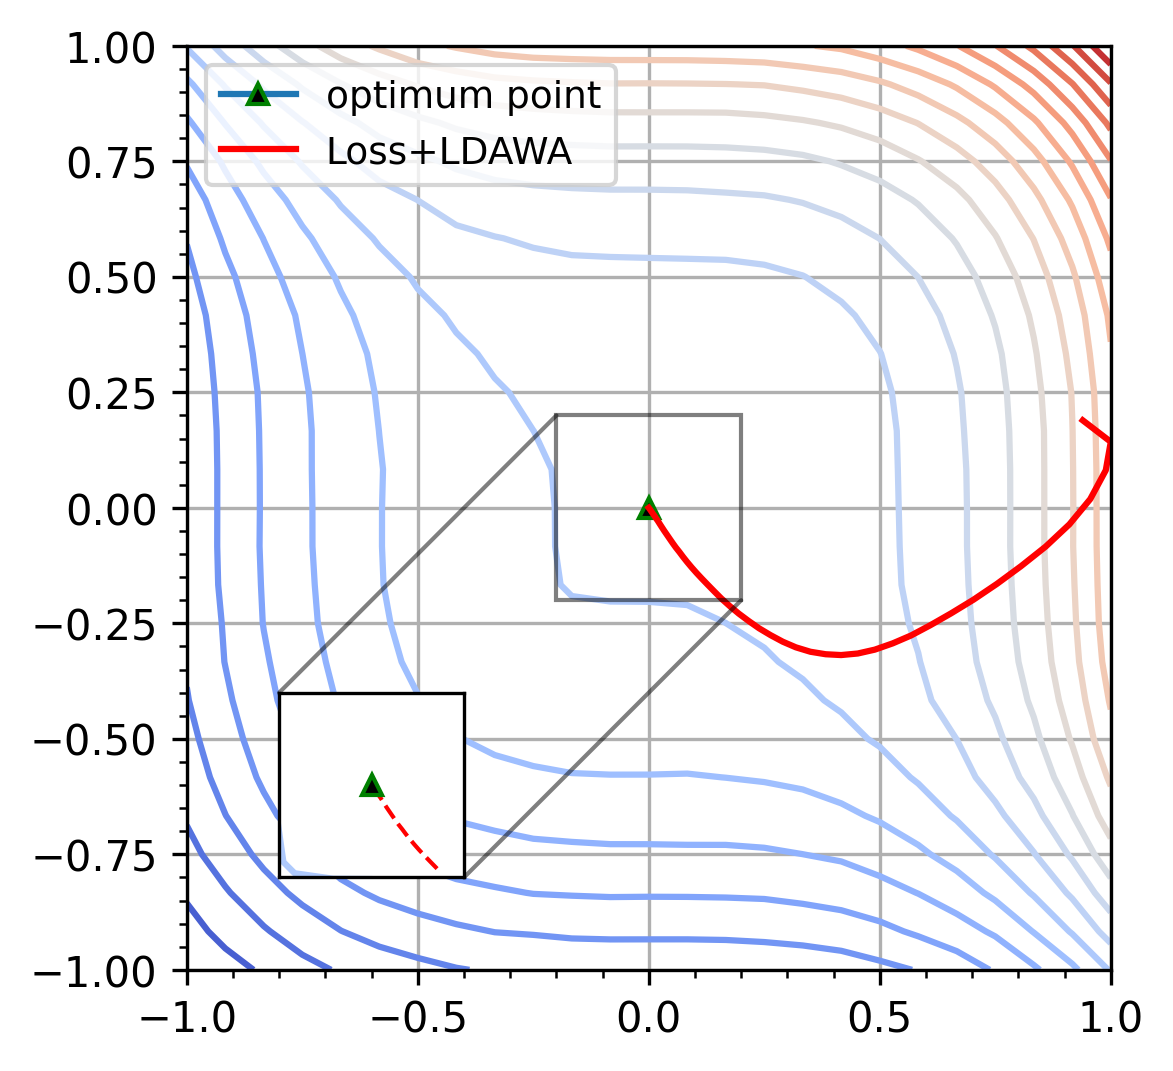}
    \caption{Loss+L-DAWA}
\end{subfigure}%
\begin{subfigure}{0.2\linewidth}
        \centering
    \includegraphics[scale=0.35]{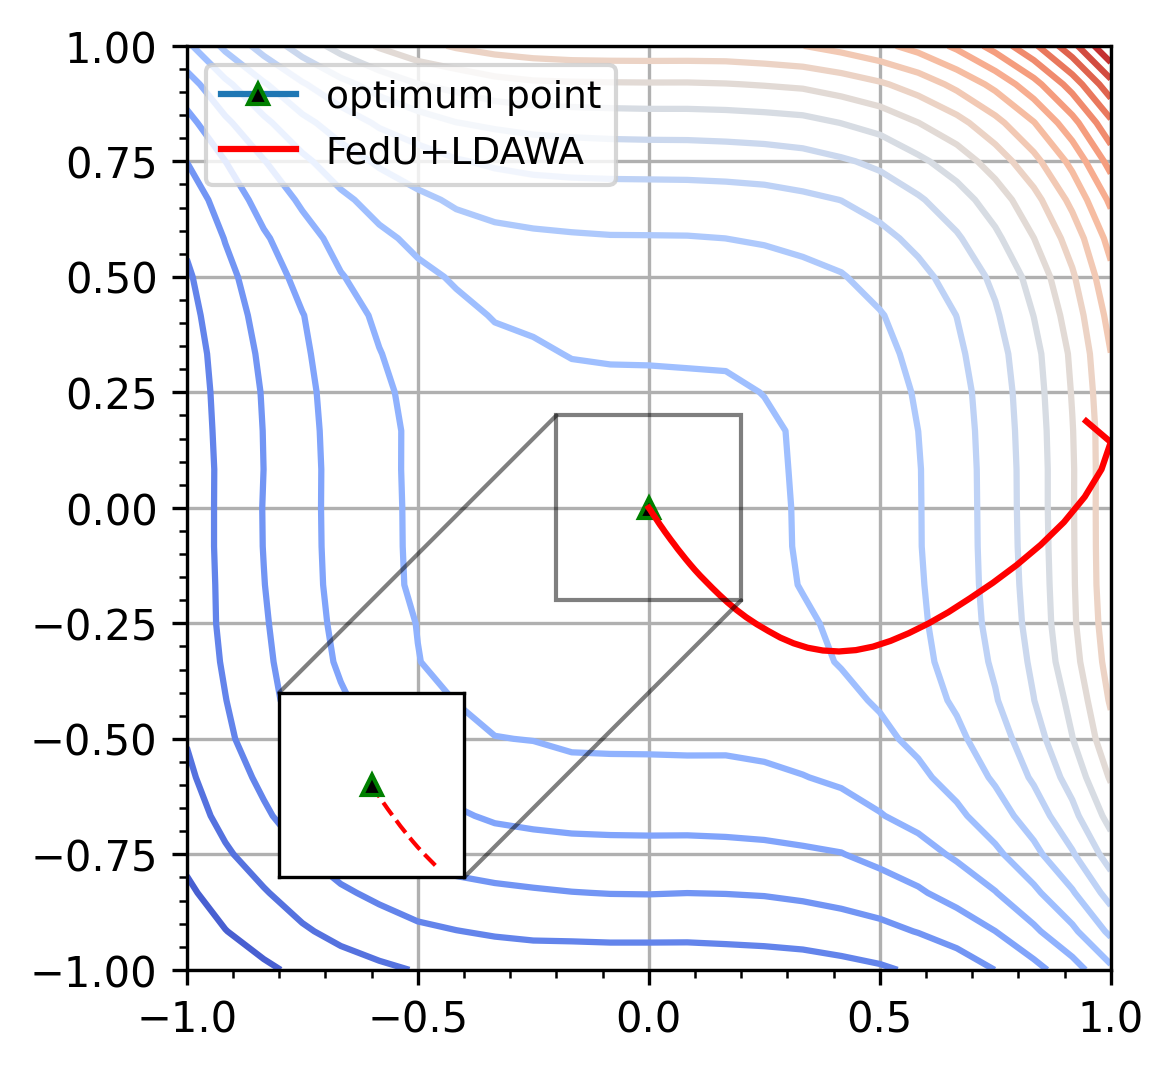}
    \caption{FedU+L-DAWA}
\end{subfigure}%
% \begin{subfigure}{0.33\linewidth}
%         \centering
%     \includegraphics[width=\linewidth]{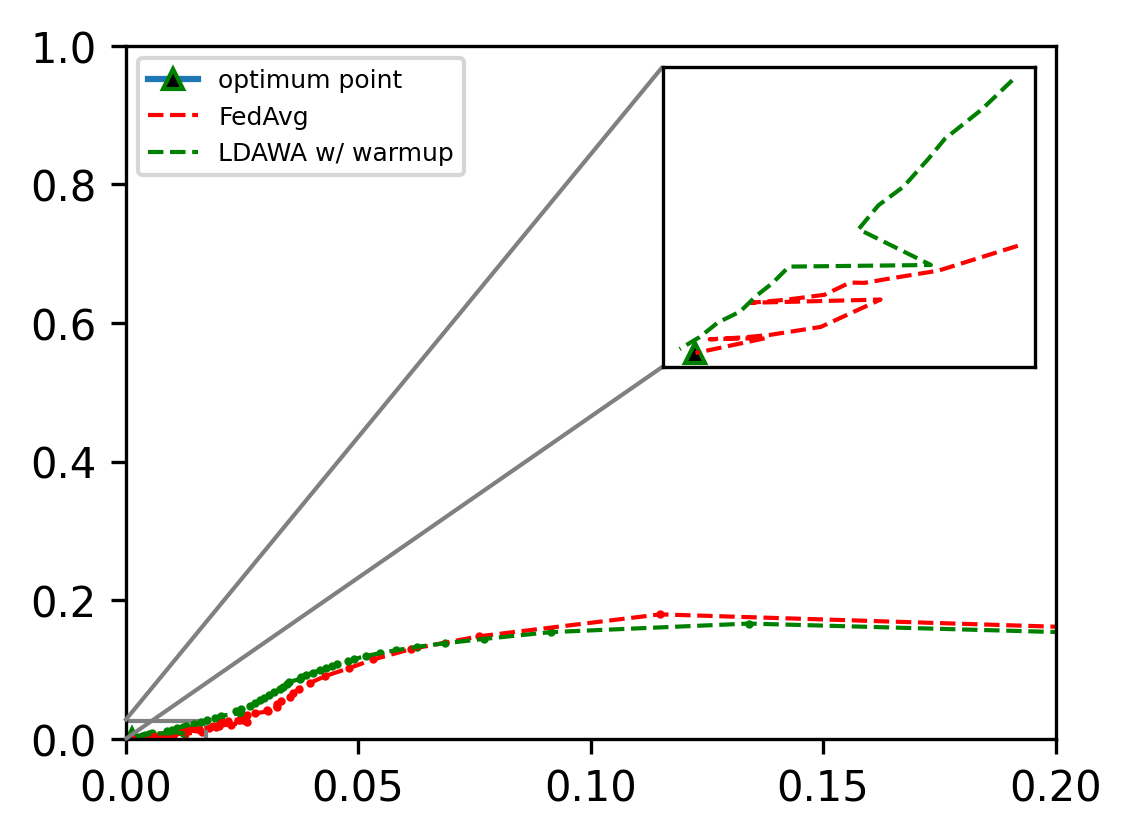}
%     \caption{Local Epochs Per Round =10}
% \end{subfigure}
    
    \caption{\small Illustration of global model's optimization trajectories and the loss landscape under various aggregation methods using SimCLR in FL settings.}
    \label{fig:Optimization-supp}
\end{figure*}

\subsection{L-DAWA minimizes the divergence between the clients}
We found that L-DAWA reduces the angular divergence between the clients' models and the global models during FL pretraining by scaling each client with its measure of the \textit{angular divergence} with respect to the global model. Such scaling controls the length of the step taken by the global model to reach the optimum point. For example, if the \textit{angular divergence} between a certain client's model and the global model is higher, L-DAWA will downscale the contribution of such client's model based on the extent of the divergence. This results in the global model optimization trajectory being less affected by the diverging clients, which results in improved control over the divergence of individual clients' models with respect to the global model. To provide a formal illustration, we compute the average angular divergence for each client in \textit{cross-silo} FL settings with SimCLR as shown in Figure \ref{fig:div-supp}. One can see from Figure \ref{fig:div-supp} that the \textit{angular divergence} (a.k.a cosine of the angle between the global model and client's models) of FedAvg for all clients with increasing local epochs gets higher resulting in lower values of mean angular divergence. On the other hand, L-DAWA maintains a steady angular divergence resulting in higher mean values for angular divergence.                      

\begin{figure*}
    \begin{subfigure}{0.33\linewidth}
        \includegraphics[width=\linewidth]{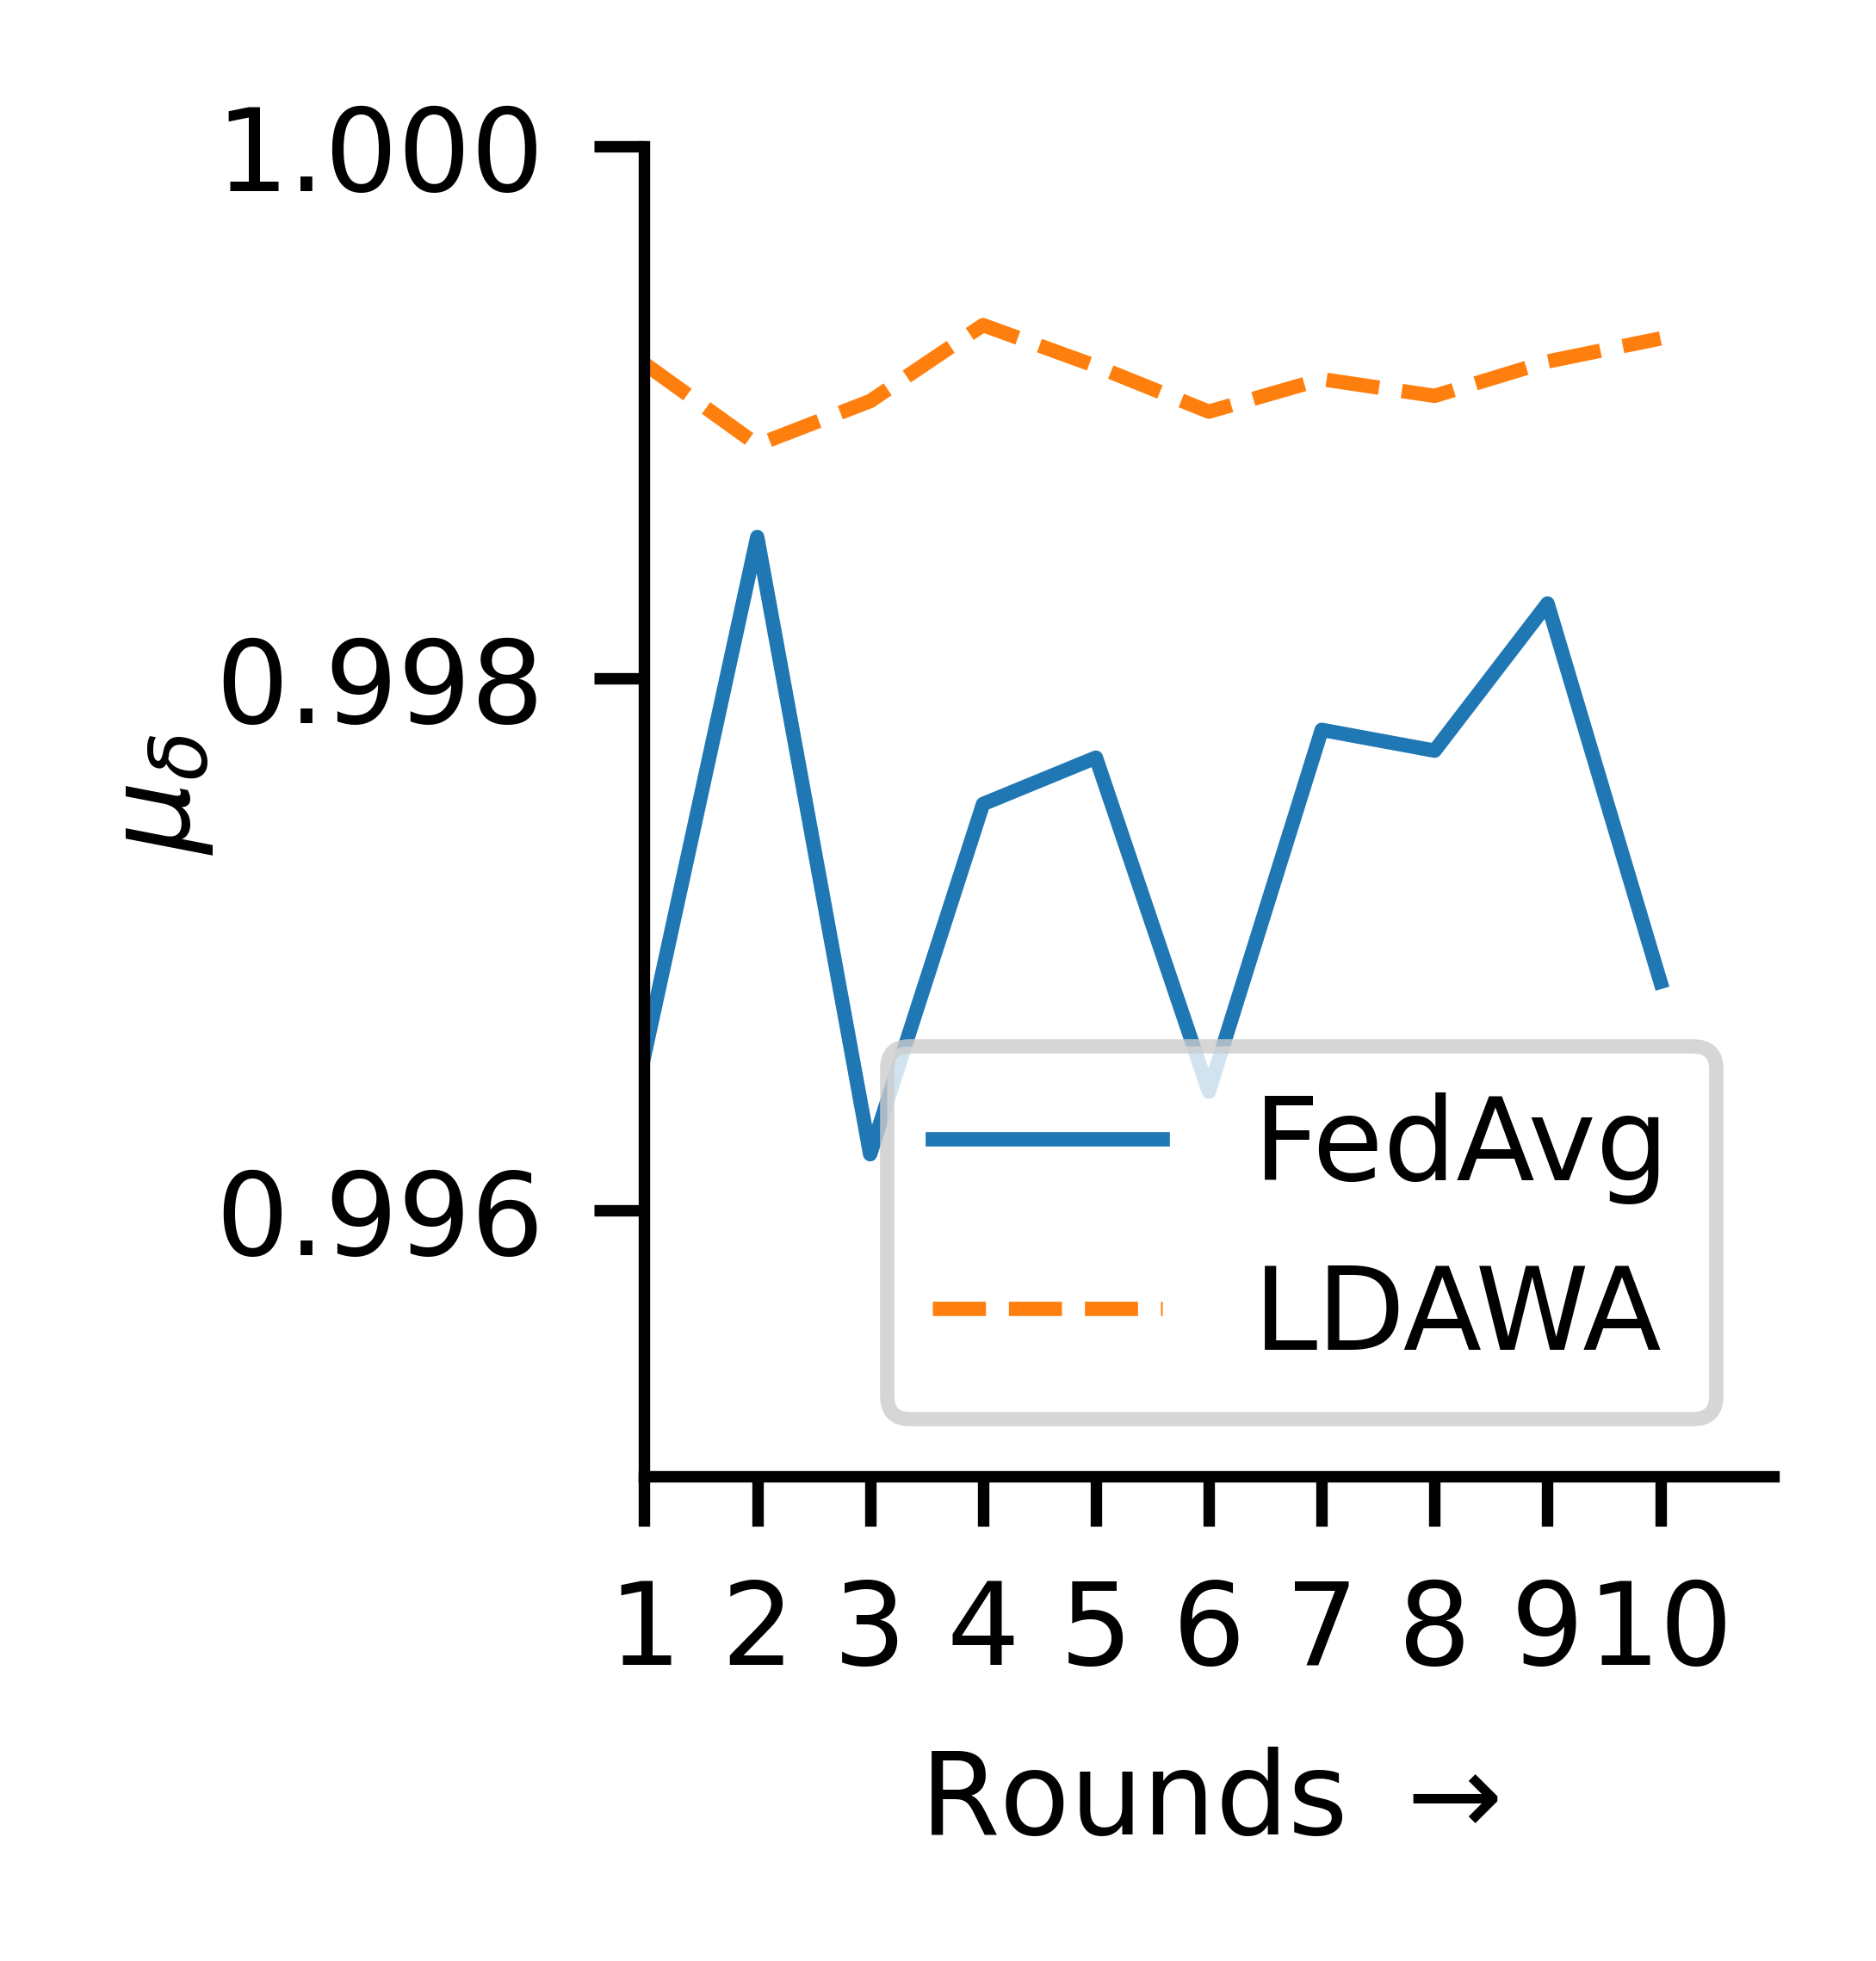}
        \subcaption{E=1}
    \end{subfigure}%
    \begin{subfigure}{0.33\linewidth}
        \includegraphics[width=\linewidth]{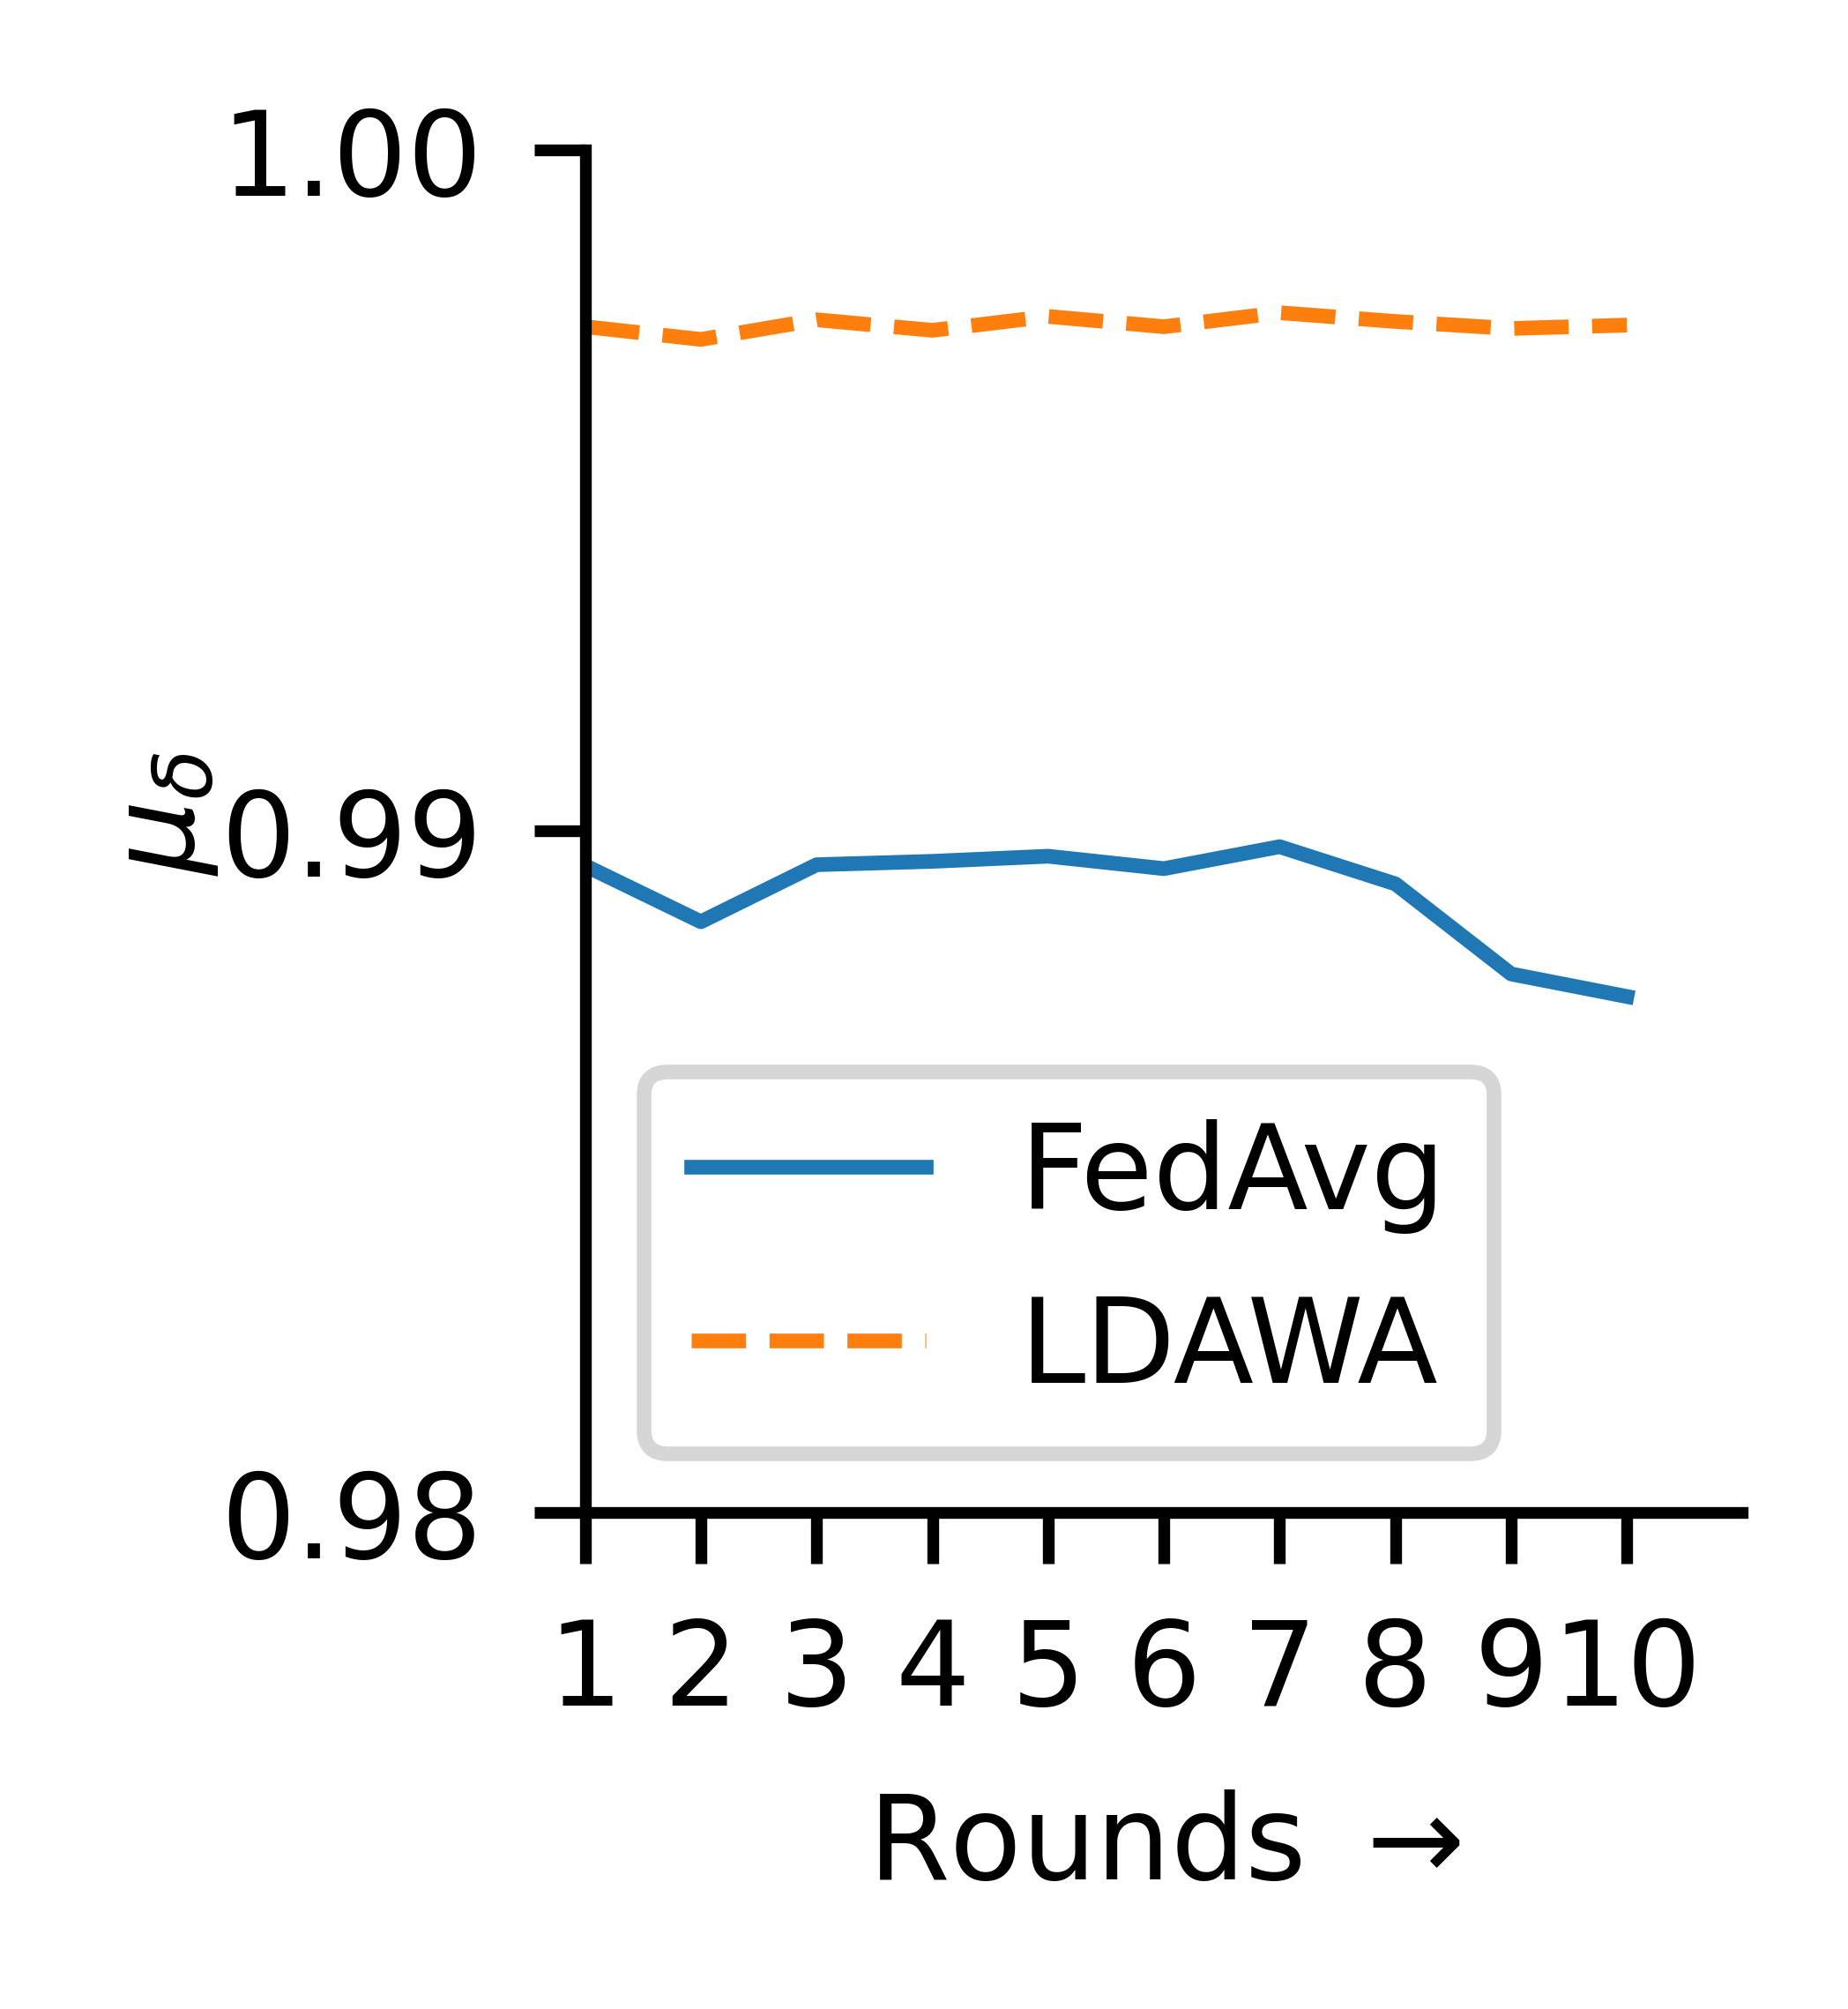}
        \subcaption{E=5}
    \end{subfigure}%
    \begin{subfigure}{0.33\linewidth}
        \includegraphics[width=\linewidth]{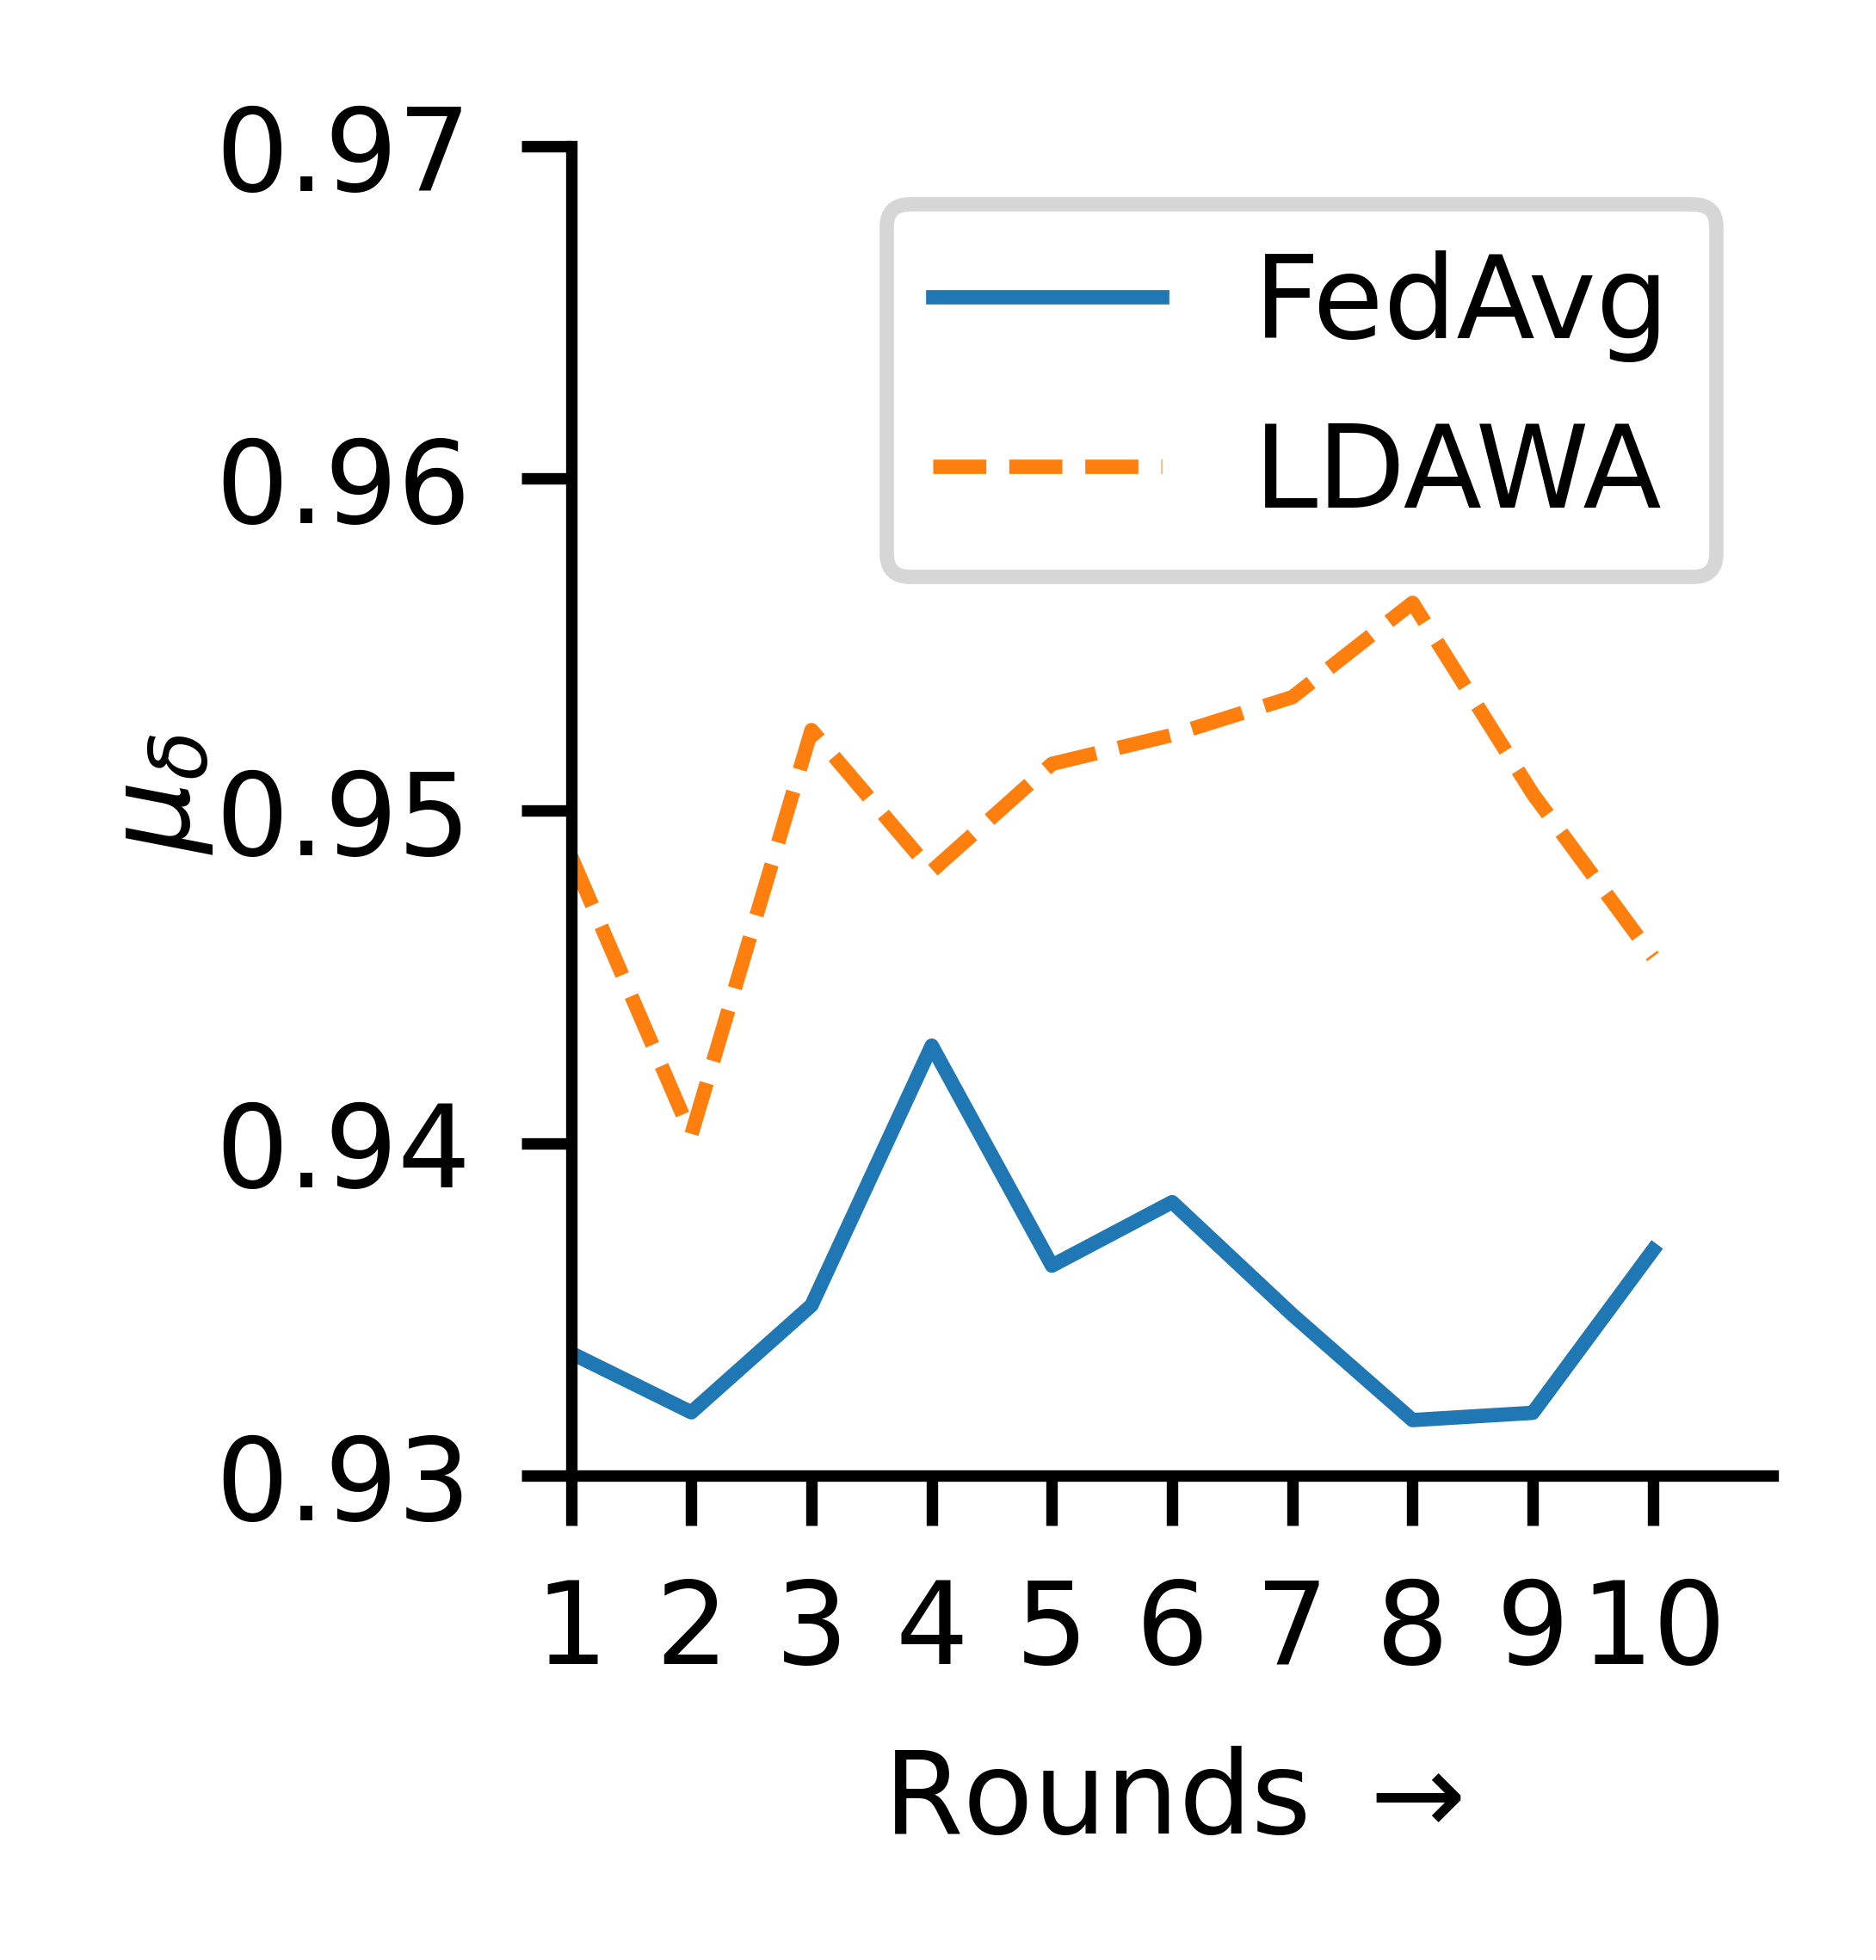}
        \subcaption{E=10}
    \end{subfigure}
   
    \caption{\small The mean angular divergence between the clients' models with respect to the previous global model averaged over $R=100$ rounds, computed by the following equation: $\mu_{\delta} = \frac{1}{R} \sum_{r=1}^{R}\delta^{r}_{k}$, where $k=\{1,...,10\}$. The higher $\delta$ value means lower divergence. L-DAWA has a good control of oscillations,  maintaining the angular divergence in a lower level over FL rounds than FedAvg.}
     \label{fig:div-supp}
\end{figure*}

\subsection{Convergence to the Same Optima}
We empirically show that L-DAWA and L-DAWA combined with FedAvg (i.e., L-DAWA$_{FedAvg}$), provide nearly the same performance on all the participating clients in FL \textit{cross-silo} settings. This phenomenon suggests that the inclusion of angular divergence measurement $\delta$ restricts the divergence bounds of the optimization trajectory in the global model. To simulate such an effect, we pre-trained a SimCLR on the Non-iid ($\alpha=0.1$) version of CIFAR10 for $R=200$ rounds under the \textit{cross-silo} settings ($K=10$) with FedAvg, L-DAWA, and L-DAWA$_{FedAvg}$. After pre-training, we fine-tune the last layer of the pre-trained global model on the individual clients' dataset that has participated in FL and subsequently evaluate it on the common CIFAR-10 test set. We show the results in Table \ref{tab:local_vs_global}. From the results of Table \ref{tab:local_vs_global}, we noted  the following observations:
\begin{enumerate}
    \item The clients with more data do not necessarily give better performance. One can see from Table \ref{tab:local_vs_global}, that the client $5,7$ contain more than $8000$ data samples, however, their performance on the test set is $32.21\%$ and $34.85\%$, respectively. In contrast, client $1$ contains $5839$ samples while obtaining a much better performance of $40.18\%$ on the test set. One can see that in the \textit{cross-silo} settings, FedAvg will prioritize client $5,7$ over other clients with a probability (weighting) of $0.18$ and $0.17$, respectively resulting in sub-optimal perforamance. On the other hand, client $1$ would only obtain a probability (weighting) of $0.11$, thus down-weighting the participation of client $1$ during FL pre-training.
    
    \item The introduction of \textit{an angular measure of divergence} in FedAvg (i.e., L-DAWA$_{FedAvg}$) resulted in similar performance as with L-DAWA, for all the clients. One can see from Table \ref{tab:local_vs_global}, that clients aggregation with L-DAWA and L-DAWA$_{FedAvg}$ show similar results suggesting $\delta$ effectively reduces the divergence, the effects of biased-weighting of FedAvg, and controls the optimization trajectory. We conjecture that this is due to L-DAWA and L-DAWA$_{FedAvg}$ trajectories being closer to each other in the optimization surface. On average, one can see that the introduction of $\delta$ in FedAvg provides nearly $2.45$\% gain in the performance across the clients. 
\end{enumerate}

\begin{table*}[ht]
    \centering
    \resizebox{2\columnwidth}{!}{
    \begin{tabular}{c|cccccccccc|c}
    \hline
         client $\rightarrow$ & 1 & 2 & 3 & 4 & 5 & 6 & 7 & 8 & 9 & 10 & Avg \\
         \hline
          Data Samples per client $\rightarrow$ & 5839 & 163 & 2477 & 5706 & 8780 & 7183 & 8519 & 6518 & 2978 & 1802 & 4996.5 \\
         \hline
         FedAvg & 40.18 & 27.22 & 23.64 & 30.55 & 32.21 & 41.89 & 34.85 &39.22 & 18.92 & 27.65  & 31.63\\
         \hline
         L-DAWA & 42.57 & 29.97 & 26.95 & 32.64 & 33.68 & 45.02 & 36.74 & 43.58 & 19.69 & 29.93 & \textbf{34.08} \\
         L-DAWA$_{FedAvg}$ & 43.13 & 30.63& 26.96 & 33.00 &33.68 & 45.61 & 38.21 & 43.62 & 20.07 & 30.19 & \textbf{34.51}\\
         \hline
    \end{tabular}
    }
    \caption{Linar-probe accuracy of the FL (cross-silo) pre-trained model. After FL pre-training, we fine-tune the last layer of each client model with the client's local dataset and evaluate it on the CIFAR-10 test set. It can be seen that L-DAWA and L-DAWA$_{FedAvg}$ provide nearly the same test results suggesting that both L-DAWA and L-DAWA$_{FedAvg}$ may converge to the similar basin of loss landscape  during FL pre-training.}
    \label{tab:local_vs_global}
\end{table*}

\subsection{Comparison with SOTA FL Aggregation Methods}
\textcolor{blue}{We compare L-DAWA with FedAvg\cite{mcmahan2017communication}
, Loss\cite{gao2022end}, FedU\cite{zhuang2021collaborative}, and EUC \cite{lee2021layer} in Table \ref{tab:EUC_vs-DAWA-C}. For the EUC method, we use the 'layer-wise unit model discrepancy' measure to make a decision about the update of the global model's layer with the client's model layer during aggregation. }

\begin{table}[ht]
    \centering
    
    \scalebox{0.8}{
    \begin{tabular}{lcccccc}
    \toprule
        & \multicolumn{3}{c}{SimCLR} & \multicolumn{3}{c}{Barlow Twins} \\
        \hline
         Method & E=1 & E=5 & E=10 & E=1 & E=5 & E=10\\
         \hline
         FedAvg (Baseline)  &  50.92 & 65.42 & 71.07 & 51.65 & 58.84 & 65.02\\
         Loss \cite{gao2022end} & 50.99 & 63.83 & 71.34 & 48.24 & 54.64 & 57.12 \\
         FedU \cite{zhuang2021collaborative} &  51.35 & 64.63 & 70.36 & 50.60 & 58.26 & 64.55\\
         EUC \cite{lee2021layer} & 51.23 & 64.10 & 70.51 & 51.16 & 58.76 & 63.60 \\
         \hline
         L-DAWA & \textbf{60.29} & \textbf{70.65} & \textbf{75.60} & \textbf{54.84} & \textbf{65.07}&\textbf{69.31}\\
         
        %  L-DAWA-WA & \xmark & None & 50.05 & 61.29  & 66.58 \\
        %  L-DAWA  & \xmark & None & \textbf{54.21} & \textbf{64.75} & \textbf{68.73}\\
        
        %  L-DAWA (w/o $w^{r-1}_{g}$) & \xmark & None & 55.13 & 65.61 & 69.05 \\
        %  L-DAWA-W$_{FedAvg}$  & \cmark & Data Samples  & \textbf{55.30} & \textbf{67.14} & \textbf{70.22}  \\
         \bottomrule
    \end{tabular}
    }
    \caption{\small Ablation study: Linear-probe accuracy on downstream task and average aggregation execution time for FedAvg, FedU, and EUC. Each method is pre-trained with SimCLR on the Non-iid version ($\alpha$=0.1) of CIFAR-10 for R=200 rounds under the \textit{cross-silo (K=10)} settings.}
    \label{tab:EUC_vs-DAWA-C}
    \vspace{-5mm}
\end{table}

\subsection{Evaluation on federated supervised training}
Our proposed method has the potential to be extended to the setting of federated supervised training. We conduct an evaluation on the Non-iid version of CIFAR-10 under \textit{cross-silo} (K=10) setting. One can see from Table \ref{tab:supervised} that L-DAWA surpasses all other baseline methods by at most $1.41$\%.

\begin{table}[ht]
    \centering
    
    \scalebox{1}{
    \begin{tabular}{lccc}
    \toprule
         Aggregation Type & E1 & E5 & E10 \\
         \hline
             FedAvg  & 77.91 & 83.76 & 81.31 \\
        
             FedYogi  & 77.49 & 72.50  & 74.85 \\
        
             FedProx  & 80.55 & 74.87 & 72.24 \\
        \hline
             L-DAWA  & \textbf{81.96} & \textbf{84.68} & \textbf{82.35} \\
    \bottomrule
    \end{tabular}
    }
    \caption{\small Supervised evaluation on the Non-iid version of CIFAR-10 under the \textit{cross-silo (K=10)} settings. The models are trained for $500$, $100$ and $50$ FL rounds corresponding to the settings of $1$, $5$ and $10$ local epoch(s), respectively.  }
    \vspace{-4mm}
    \label{tab:supervised}
\end{table}

\subsection{Linear Fine-tuning on Cross-Device Setting}
Although our analysis is mostly limited to the \textit{cross-silo} settings, we also provide results for the more challenging \textit{cross-device} settings. Table \ref{tab:comp_sota_cross-device-appendix} shows that our proposed methods still obtain the best performance in most of setup, except for the $10$\% training data settings on CIFAR-100 dataset. Especially, L-DAWA achieves significant gains in the extreme semi-supervised settings with only $1$\% training data on CIFAR-100. Additionally, when layer-wise divergence is introduced in FedAvg, Loss, and FedU, we see a performance improvement in most of the cases, as shown in Table \ref{tab:comp_sota_cross-device-appendix}, suggesting the importance of the integration of divergence into aggregation within \textit{cross-device} setting.

\begin{table*}[ht]
    \centering
    \resizebox{2\columnwidth}{!}{
    \begin{tabular}{l|c|c|c|c|c|c|c|c|c|c|c|c}
         \toprule
        %  \multicolumn{13}{|c|}{Cross-Device}\\
        %  \hline
         \multirow{3}{*}{Method}& \multicolumn{6}{c}{CIFAR-10} & \multicolumn{6}{c}{CIFAR-100}\\
         \cline{2-13}
         &  \multicolumn{3}{c}{SimCLR} & \multicolumn{3}{c}{Barlow Twins} & \multicolumn{3}{c}{SimCLR} & \multicolumn{3}{c}{Barlow Twins}\\
        \cline{2-13}
        & 100\% & 1\% & 10\% & Linear&  1\% & 10\%  & 100\%  &   1\% & 10\%   & 100\%  &   1\% & 10\%  \\
        \cline{2-13}
         \hline
         FedAvg   & 68.66 & 52.83 & 66.22 & 62.07 & 44.50 & 57.60 &  44.59 & 14.18  &\textbf{32.55} & 32.65 & 8.53 & 20.85 \\
          Loss   & 66.09 & 48.93 & 63.24 & 56.40 & 40.31 & 52.02 & 44.83 & 14.05 & 32.40 &  33.27 & 9.11  & \textbf{21.88} \\
          FedU    & 68.52 & 51.52 & 66.20 & 61.43 & 45.17 & 57.01 & 44.56 & 13.54 & 31.86 & 32.89 & 9.06 & 21.61 \\
         \hline
        %  L-DAWA    & 67.02 & 47.23 & 62.13 & 51.62 & 34.58 & 44.65 &  41.83 & 11.53 & 28.65 & 27.84 & 7.05& 17.00  \\
        L-DAWA    & 68.20 & 51.45 & 64.71 & 58.25 & 41.86 & 53.26 & 45.04  &  \textbf{14.64} & 32.07  & \textbf{34.12} & \textbf{9.39} & 21.84   \\
        L-DAWA$_{FedAvg}$  & \textbf{69.92} & 52.15 & 65.73 & \textbf{62.32} & 44.75 & 56.93 & 44.19 & 13.79 &  31.80 & 33.20  & 8.46 & 21.78 \\
        L-DAWA$_{Loss}$ & 68.79 & \textbf{53.66} & 65.68 & 61.36 &  44.77 &56.88  & \textbf{45.08} & 14.63 & 31.67 & 31.93 &  8.40 & 20.25 \\
        L-DAWA$_{FedU}$  &  69.69 &  52.41 & \textbf{66.63} & 62.19 & \textbf{46.64} & \textbf{58.46} & 44.97 & 14.05 & 31.85 & 32.84 & 8.95 & 21.07\\
        %   L-DAWA-ver1    & 66.25 &  47.55 &  & 55.50 &  & 37.87      &   &  &  &  & &   \\
         \bottomrule
    \end{tabular}
    }
    \caption{Comparison of the proposed aggregation strategy with state-of-the-art methods on CIFAR-10 and CIFAR-100 under \textit{cross-device (K=100)} settings.}
    \label{tab:comp_sota_cross-device-appendix}
\end{table*}

\subsection{Transfer Learning under Cross-Device Settings}
We further evaluate the generalization of the learned features from FL pre-training by fine-tuning the resulting model on a different dataset. Such evaluation helps in assessing whether the pre-trained features can be transferred to different downstream tasks. We follow the same procedure that is adopted for linear evaluation. Specifically, we first perform FL pre-training on CIFAR-10 (CIFAR-100) followed by linear-probe (fine-tuning the last classification layer) on CIFAR100 (CIFAR10). Note that the  CIFAR-10 classes and CIFAR-100 classes are mutually exclusive \cite{krizhevsky2009learning}.   

One can see from Table \ref{tab:Transfer Learning}, that L-DAWA generalizes well for both SimCLR and Barlow Twins compared to other aggregation strategies in the \textit{cross-device} settings. We further show that when the layer-wise divergence is introduced in FedAvg, Loss, and FedU, we find a performance improvement for these methods in most of the cases in \textit{cross-device} settings.

\begin{table}[ht]
    \centering
    \resizebox{\columnwidth}{!}{
    \begin{tabular}{l|cc|cc}
    \toprule
        & \multicolumn{4}{|c}{Cross-Device}\\
        \cline{2-5}
        &  \multicolumn{2}{|c|}{CIFAR-10 $\rightarrow$ CIFAR-100}& \multicolumn{2}{|c}{CIFAR-100 $\rightarrow$ CIFAR-10}\\
         \hline
         Method &  SimCLR & Barlow Twins & SimCLR & Barlow Twins  \\
         \hline
        %  \cline{2-5}
         FedAvg &  44.94 & 37.77 & 67.48 &\textbf{57.71}\\
         Loss & 41.33 & 32.06 & 66.91 & 56.61 \\
         FedU & 44.28 & 37.21 & 67.12 & 56.53\\
        %  L-DAWA & \underline{45.60} & \underline{39.29} & \underline{73.59} & \underline{66.39}& 41.58 & 26.71 & 65.91 & 52.15\\
         \hline
         L-DAWA & 43.65 & 33.51 & \textbf{68.21}  & 57.66\\

         L-DAWA$_{FedAvg}$ & \textbf{45.28} & 36.88 & 67.01 & 57.45\\
         L-DAWA$_{Loss}$ &  45.07 & 37.18 & 67.99 & 55.55\\
        %  L-DAWA$_{FedU}$ & \textbf{45.53} & \textbf{38.10}& \textbf{74.04}& \textbf{63.08} & 43.02 & 31.01 & &\\
         L-DAWA$_{FedU}$ & 45.10 & \textbf{38.08} & 67.69 & 56.73 \\
         
        %  Centralized &51.17 & & & \\
    \bottomrule
    \end{tabular}
    }
     \caption{Transfer learning under the \textit{cross-device} settings.}
    \label{tab:Transfer Learning}
\end{table}

\subsection{Effects of Momentum}
We provide an ablation study in Table \ref{tab:momentum} to highlight the importance of SGD momentum during FL pre-training. In short, we find that turning on the SGD momentum for Barlow Twins during FL pre-training can adversely affect the downstream task performance. In contrast, SimCLR improves the downstream task performance by turning on the SGD momentum during FL pre-training. We conjecture that this is due to the less divergence caused by SimCLR compared to Barlow Twins in FL settings.

\begin{table}[ht]
    \centering 
    \resizebox{\linewidth}{!}{
    \begin{tabular}{l|lcccc}
        \toprule
        Agg.strategy & SSL-Method & Momentum & E1 & E5 & E10 \\
        \hline
        \multirow{4}{*}{FedAvg} & F-SimCLR & \cmark & \textbf{51.29} & \textbf{68.25} & \textbf{74.50}\\
        & F-Barlow Twins & \cmark & \textbf{57.49} & 63.49 & 66.56 \\ 
        \cline{2-6}
         & F-SimCLR & \xmark & 49.05 & 59.52 & 66.36 \\
         & F-Barlow Twins & \xmark & 53.36 & \textbf{65.89} & \textbf{68.03} \\ 
          \hline
        
         \multirow{2}{*}{Centralized}& SimCLR & \cmark & \multicolumn{3}{c}{\textbf{85.27}}\\
         & Barlow Twins & \cmark & \multicolumn{3}{c}{\textbf{81.55}}\\
         \bottomrule
    \end{tabular}
    }
    \caption{Momentum Analysis: Linear evaluation accuracy on the CIFAR10 dataset with \textit{cross-silo} settings and iid data.}
    \label{tab:momentum}
     
\end{table}

\subsection{Effects of Warm-up}
We found that performing a few rounds of warm-up with FedAvg before starting FL training with LDAWA as an aggregation strategy provides a better initialization point for SimCLR with 10 local epochs per round and for Barlow Twins with 1,5 and 10 local epochs per round. To keep the consistency in the experiments, we perform a warm-up for 2 rounds of FedAvg before starting FL pretraining with L-DAWA.

\begin{table}[ht]
    \centering
    \resizebox{\linewidth}{!}{
    \begin{tabular}{lcccccc}
    \toprule
         & \multicolumn{3}{c}{SimCLR} & \multicolumn{3}{c}{Barlow Twins}\\
         Aggregation Type & E1 & E5 & E10 & E1 & E5 & E10 \\
        \hline
        L-DAWA (w/o warm-up)  & \textbf{62.71} & \textbf{71.16} & 75.49 & 49.41 & 62.65 & 68.64 \\
        L-DAWA (w/ warm-up)  & 60.29 & 70.65 & \textbf{75.60} & \textbf{54.84}  &\textbf{ 65.07} &  \textbf{69.31} \\
    \bottomrule
    \end{tabular}
    }
    \caption{\small Performance of LDAWA with (w) and without (w/o) warm-up round. We use FedAvg for aggregation during the warm-up round. }
    \vspace{-4mm}
    \label{tab:warmup}
\end{table}

\begin{table}[ht]
    \centering
    \begin{tabular}{c|c|c|c|c|c|c}
    \hline
         Method & \multicolumn{3}{c}{SimCLR} & \multicolumn{3}{c}{Barlow Twins} \\
         \hline
         & 100\% & 1\% & 10\% & 100\% & 1\% &10\% \\
         \hline
         FedAvg & 32.92 & 12.66 & 24.54 & 15.40 & 5.21 & 11.35\\
         Loss &33.37& 12.77 & 24.12 &  12.24 &3.14 & 6.72 \\
         FedU &32.63 & 12.11 &24.23 &15.16 & 5.29 &10.49  \\
         \hline
         L-DAWA & \textbf{37.22}& 12.74 & \textbf{26.31} & \textbf{21.47}& \textbf{8.20} & \textbf{15.19}\\
         \hline
    \end{tabular}
    \caption{Results on Tiny ImageNet}
    \label{tab:my_label}
\end{table}
